# Supplementary material for: Improved Modelling of Detector Response Effects in Phonon-based Crystal Detectors used for Dark Matter Searches
Source: arXiv:2403.01259 ancillary file (2024-06-24)
Supplement: Supplementary file 1 [file Catalog_of_CTII_Solutions.pdf]

# Catalog of single-electron-hole-pair solutions for the exponential charge trapping and impact ionization model

M. J. Wilson <sup>\*1</sup>, A. Zaytsev<sup>1</sup>, and B. von Krosigk<sup>2</sup>

<sup>1</sup>Institut für Astroteilchenphysik, Karlsruher Institut für Technologie, 76133 Karlsruhe, Germany

<sup>2</sup>Kirchhoff-Institut für Physik, Universität Heidelberg, 69117 Heidelberg, Germany

March 2, 2024

## 1 Introduction

This document provides a catalog of the unique analytical solutions found for the charge trapping (CT) and impact ionization (II) exponential model. There are three classes of events in which solutions are found: surface events (Sec. 2), bulk-single-charge events (Sec. 3), and bulk-electron-hole ( $e^-h^+$ )-pair events (Sec. 4). Section 5 describes how these solutions can be accessed from a Python file that is also provided as supplement material. The main article provides a description on how these solutions are established and solved for; this document provides only the final solutions. Results published using these solutions or the provided Python file must include the citation of the main article.

All of the solutions are written as a function of ionization energy  $E$ , where  $E$  is in the  $n_{\text{eh}}$ -energy space (denoted as  $E_{\text{neh}}$  in the main article). The other parameters in the solutions include  $\tau$  and  $T$  parameters. The  $\tau$  parameters represent a characteristic length of a particular process. If a process  $i$  has a fractional probability of  $f_i$  for a charge travelling the length of the detector, then the characteristic length  $\tau_i$  is given by:

$$\tau_i = \frac{-1}{\ln(1 - f_i)}. \quad (1)$$

For electrons,  $i = \text{“CTe”}$  (trapping),  $\text{“IIee”}$  (creation of an unpaired electron), or  $\text{“IIeh”}$  (creation of an unpaired hole). For holes,  $i = \text{“CTh”}$  (trapping),  $\text{“IIhh”}$  (creation of an unpaired hole), or  $\text{“IIhe”}$  (creation of an unpaired electron). The  $T$  parameters defined for each charge are given by:

$$\begin{aligned} T_{\text{e}} &\equiv \frac{1}{\tau_{\text{CTe}}} + \frac{1}{\tau_{\text{IIee}}} + \frac{1}{\tau_{\text{IIeh}}} \\ T_{\text{h}} &\equiv \frac{1}{\tau_{\text{CTh}}} + \frac{1}{\tau_{\text{IIhh}}} + \frac{1}{\tau_{\text{IIhe}}}. \end{aligned} \quad (2)$$

## 2 Surface events

Surface events assume that the initial starting position of a charge (either  $e^-$  or  $h^+$ ) is at one of the surfaces of the detector. The general solutions for specific scenarios are the same whether the initial charge is an  $e^-$  or a  $h^+$ . What is only required is the distinction between parameters associated with the initial

---

\*matthew.wilson@kit.edu

charge (parameters labelled with “s”) and parameters associated with the opposing charge (parameters labelled with “o”). The solutions for surface events are found up to second-order scenarios. That means that charges that participated or were produced in a primary II process can take part in no more than one additional II processes. Charges existing after the maximum number of II processes propagate to a crystal surface with 100 % probability.

Each solution below provides a text description of the scenario, an illustration of the scenario, the combinatorial factor, and the unique analytical solution. In come cases, different solutions are required in the case where the  $T$  parameters are the same for electrons and holes. Also note that the combinatorial factor is already accounted for in the solutions provided.

The illustrations can be read as follows. The black, vertical bars represent the crystal surfaces. Electrons are represented by blue, solid lines and propagate from left to right. Holes are represented by red, dashed lines and propagate from right to left. An open circle indicates that a charge is trapped, and a diamond indicates a charge has created another charge. The initial charge has the darkest shade, with charges existing after an occurrence of II having an increasingly lighter shade. The illustrations show both scenarios for when the initial charge is either an  $e^-$  or a  $h^+$ .

### Solution 0

**Description:** Electron (hole) reaches the surface.

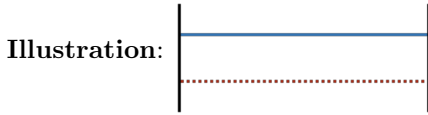

**Combinatorial factor:** 1

**Solution:**

$$P_0(E) = \delta(E - 1) e^{-T_s}$$

### Solution 1

**Description:** Electron (hole) traps.

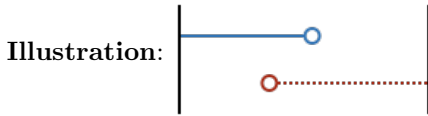

**Combinatorial factor:** 1

**Solution:**

$$P_1(E) = \begin{cases} \frac{1}{\tau_{CTs}} e^{-T_s \cdot E} & 0 \leq E < 1 \\ 0 & \text{else} \end{cases}$$

### Solution 2

**Description:** Electron (hole) creates an electron (hole).

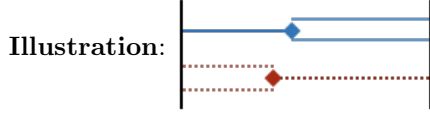

Combinatorial factor: 1

Solution:

$$P_2(E) = \begin{cases} \frac{1}{\tau_{1\text{Iss}}} e^{-T_s \cdot E} & 1 \leq E < 2 \\ 0 & \text{else} \end{cases}$$

### Solution 3

**Description:** Electron (hole) creates a hole (electron).

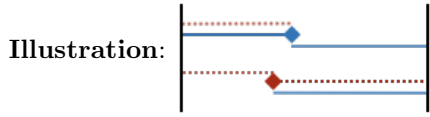

Combinatorial factor: 1

Solution:

$$P_3(E) = \begin{cases} \frac{1}{\tau_{1\text{Iso}}} e^{T_o - T_s - T_o \cdot E} & 1 \leq E < 2 \\ 0 & \text{else} \end{cases}$$

### Solution 4

**Description:** Electron (hole) creates an electron (hole). One electron (hole) traps.

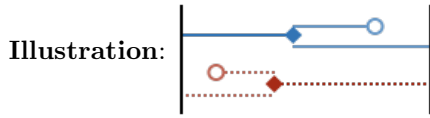

Combinatorial factor: 2

Solution:

$$P_4(E) = \begin{cases} \frac{2e^{-T_s \cdot E}}{\tau_{1\text{Iss}} \tau_{CTs}} (2 - E) & 1 \leq E < 2 \\ 0 & \text{else} \end{cases}$$

### Solution 5

**Description:** Electron (hole) creates an electron (hole). Both electrons (holes) trap.

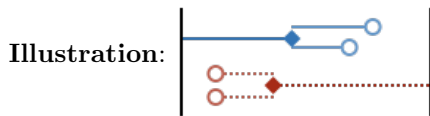

Combinatorial factor: 1

**Solution:**

$$P_5(E) = \begin{cases} \frac{e^{-T_s E}}{2\tau_{\text{Iso}}\tau_{t,s}^2} E^2 & 0 \leq E < 1 \\ \frac{e^{-T_s E}}{2\tau_{\text{Iso}}\tau_{t,s}^2} (E-2)^2 & 1 \leq E < 2 \\ 0 & \text{else} \end{cases}$$

## Solution 6

**Description:** Electron (hole) creates a hole (electron). The electron (hole) traps.

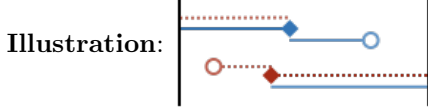

**Combinatorial factor:** 1

**Solutions:**

$$P_6(E | T_s \neq T_o) = \begin{cases} \frac{e^{-T_s E} - e^{-1/2(T_o + T_s)E}}{(T_o - T_s)\tau_{\text{Iso}}\tau_{CTs}} & 0 \leq E < 1 \\ \frac{-e^{-1/2(T_o + T_s)E} + e^{T_o - T_s - T_o E}}{(T_o - T_s)\tau_{\text{Iso}}\tau_{CTs}} & 1 \leq E < 2 \\ 0 & \text{else} \end{cases}$$

$$P_6(E | T_s = T_o) = \begin{cases} \frac{e^{-T \cdot E}}{2\tau_{\text{Iso}}\tau_{CTs}} E & 0 \leq E < 1 \\ \frac{e^{-T \cdot E}}{2\tau_{\text{Iso}}\tau_{CTs}} (2 - E) & 1 \leq E < 2 \\ 0 & \text{else} \end{cases}$$

## Solution 7

**Description:** Electron (hole) creates a hole (electron). The hole (electron) traps.

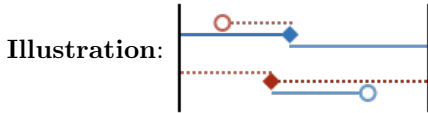

**Combinatorial factor:** 1

**Solution:**

$$P_7(E) = \begin{cases} \frac{e^{-T_s + T_o(1-E)}(2-E)}{\tau_{CTo}\tau_{\text{Iso}}} & 1 \leq E < 2 \\ 0 & \text{else} \end{cases}$$

## Solution 8

**Description:** Electron (hole) creates a hole (electron). Both the electron and hole trap.

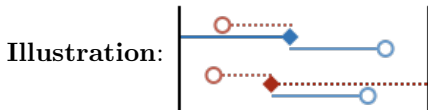

**Combinatorial factor:** 1

**Solutions:**

$$P_8(E | T_s \neq T_o) = \begin{cases} \frac{e^{-T_s E} \left( -2 + 2e^{\frac{1}{2}(-T_o + T_s)E} + T_o E - T_s E \right)}{\tau_{CTo}(T_o - T_s)^2 \tau_{Iso} \tau_{CTs}} & 0 \leq E < 1 \\ \frac{e^{-\frac{3T_o E}{2} - \frac{1}{2}T_s(2+E)} \left( 2e^{T_s + T_o E} + e^{T_o + \frac{1}{2}(T_o + T_s)E} (T_s(E-2) - 2 - T_o(E-2)) \right)}{\tau_{CTo}(T_o - T_s)^2 \tau_{Iso} \tau_{CTs}} & 1 \leq E < 2 \\ 0 & \text{else} \end{cases}$$

$$P_8(E | T_s = T_o) = \begin{cases} \frac{e^{-T \cdot E} E^2}{4\tau_{CTo} \tau_{Iso} \tau_{CTs}} & 0 \leq E < 1 \\ \frac{e^{-T \cdot E} (-2+E)^2}{4\tau_{CTo} \tau_{Iso} \tau_{CTs}} & 1 \leq E < 2 \\ 0 & \text{else} \end{cases}$$

### Solution 9

**Description:** Electron (hole) creates an electron (hole). One electron (hole) creates an electron (hole).

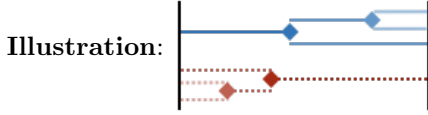

**Combinatorial factor:** 2

**Solution:**

$$P_9(E) = \begin{cases} \frac{e^{-T_s} - e^{-T_s E}}{T_s \tau_{Iso}^2} & 1 \leq E < 2 \\ \frac{e^{-T_s} - e^{-4T_s + T_s E}}{T_s \tau_{Iso}^2} & 2 \leq E < 3 \\ 0 & \text{else} \end{cases}$$

### Solution 10

**Description:** Electron (hole) creates an electron (hole). One electron (hole) creates a hole (electron).

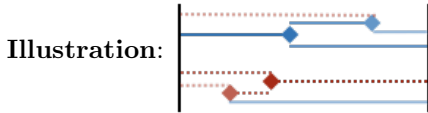

**Combinatorial factor:** 2

**Solution:**

$$P_{10}(E) = \begin{cases} -\frac{2e^{T_s - T_s E} (-3+E)}{\tau_{Iso} \tau_{Iso}} & 2 \leq E < 3 \\ 0 & \text{else} \end{cases}$$

### Solution 11

**Description:** Electron (hole) creates an electron (hole). One electron (hole) creates an electron (hole). The other electron (hole) traps.

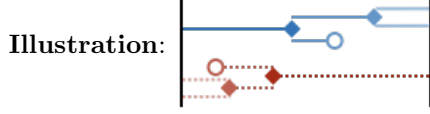

Combinatorial factor: 2

Solution:

$$P_{11}(E) = \begin{cases} \frac{e^{-T_s} \left( \sinh \left[ \frac{1}{2} (T_s - T_s E) \right]^2 + T_s (-2 + E) \sinh [T_s - T_s E] \right)}{T_s^2 \tau_{\text{IIs}}^2 \tau_{\text{CTs}}} & 1 \leq E < 2 \\ \frac{e^{-T_s} \sinh \left[ \frac{1}{2} T_s (-3 + E) \right]^2}{T_s^2 \tau_{\text{IIs}}^2 \tau_{\text{CTs}}} & 2 \leq E < 3 \\ 0 & \text{else} \end{cases}$$

### Solution 12

**Description:** Electron (hole) creates an electron (hole). One electron (hole) creates a hole (electron). The other electron (hole) traps.

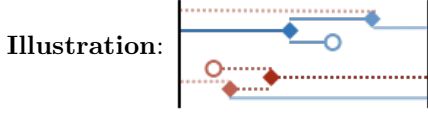

Combinatorial factor: 2

Solution:

$$P_{12}(E) = \begin{cases} \frac{e^{T_s - T_s E} (-1 + E)^2}{\tau_{\text{IIs}} \tau_{\text{IIs}} \tau_{\text{CTs}}} & 1 \leq E < 2 \\ \frac{e^{T_s - T_s E} (-3 + E)^2}{\tau_{\text{IIs}} \tau_{\text{IIs}} \tau_{\text{CTs}}} & 2 \leq E < 3 \\ 0 & \text{else} \end{cases}$$

### Solution 13

**Description:** Electron (hole) creates an electron (hole). Both electrons (holes) create an electron (hole).

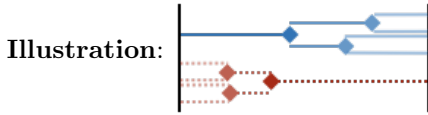

Combinatorial factor: 1

Solution:

$$P_{13}(E) = \begin{cases} \frac{e^{-T_s(1+E)} \left( e^{T_s} - 4e^{T_s E} + 3e^{\frac{1}{3} T_s (-1+4E)} \right)}{4T_s^2 \tau_{\text{IIs}}^3} & 1 \leq E < 2 \\ \frac{e^{-T_s} \left( -4 + 3e^{\frac{1}{3} T_s (-1+E)} + e^{T_s (-3+E)} (1 - 2T_s (-2+E)) \right)}{4T_s^2 \tau_{\text{IIs}}^3} & 2 \leq E < 3 \\ \frac{3e^{\frac{1}{3} T_s (-4+E)} + e^{T_s (-4+E)} (-3 + 2T_s (-4+E))}{4T_s^2 \tau_{\text{IIs}}^3} & 3 \leq E < 4 \\ 0 & \text{else} \end{cases}$$

### Solution 14

**Description:** Electron (hole) creates an electron (hole). Both electrons (holes) create a hole (electron).

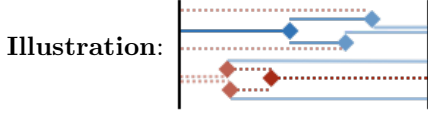

**Combinatorial factor:** 1

**Solution:**

$$P_{14}(E) = \begin{cases} \frac{e^{-T_s(-2+E)}(-2+E)^2}{2\tau_{\text{Iso}}^2\tau_{\text{IIs}}^2} & 2 \leq E < 3 \\ \frac{e^{-T_s(-2+E)}(-4+E)^2}{2\tau_{\text{Iso}}^2\tau_{\text{IIs}}^2} & 3 \leq E < 4 \\ 0 & \text{else} \end{cases}$$

### Solution 15

**Description:** Electron (hole) creates an electron (hole). One electron (hole) creates an electron (hole). The other electron (hole) creates a hole (electron).

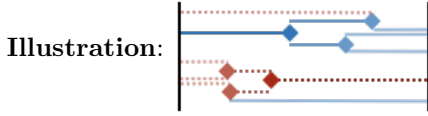

**Combinatorial factor:** 2

**Solution:**

$$P_{15}(E) = \begin{cases} \frac{e^{-T_s(1+E)} \left( (e^{2T_s} - e^{2T_s(-1+E)}) T_s(-3+E) + 2e^{T_s E} \sinh \left[ T_s - \frac{T_s E}{2} \right]^2 \right)}{T_s^2 \tau_{\text{Iso}}^2 \tau_{\text{IIs}}^2} & 2 \leq E < 3 \\ \frac{2e^{-T_s} \sinh \left[ 2T_s - \frac{T_s E}{2} \right]^2}{T_s^2 \tau_{\text{Iso}}^2 \tau_{\text{IIs}}^2} & 3 \leq E < 4 \\ 0 & \text{else} \end{cases}$$

### Solution 16

**Description:** Electron (hole) creates a hole (electron). The hole (electron) creates a hole (electron).

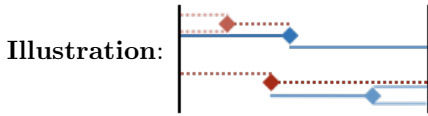

**Combinatorial factor:** 1

**Solution:**

$$P_{16}(E) = \begin{cases} \frac{e^{-T_s - T_o(1+E)}(-e^{2T_o} + e^{T_o(1+E)})}{2T_o \tau_{IIso} \tau_{IIsO}} & 1 \leq E < 2 \\ \frac{e^{-T_s - T_o(1+E)}(-e^{2T_o(-1+E)} + e^{T_o(1+E)})}{2T_o \tau_{IIso} \tau_{IIsO}} & 2 \leq E < 3 \\ 0 & \text{else} \end{cases}$$

### Solution 17

**Description:** Electron (hole) creates a hole (electron). The hole (electron) creates an electron (hole).

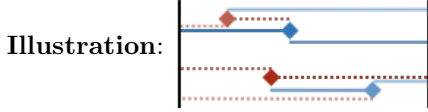

**Combinatorial factor:** 1

**Solution:**

$$P_{17}(E) = \begin{cases} \frac{e^{-T_s - T_o(-2+E)}(3-E)}{\tau_{IIso} \tau_{IIsO}} & 2 \leq E < 3 \\ 0 & \text{else} \end{cases}$$

### Solution 18

**Description:** Electron (hole) creates a hole (electron). The electron (hole) creates a hole (electron).

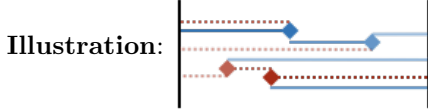

**Combinatorial factor:** 1

**Solutions:**

$$P_{18}(E | T_s \neq T_o) = \begin{cases} \frac{e^{T_s - T_o E}(-e^{(T_o - T_s)E} + e^{\frac{1}{2}(T_o - T_s)(1+E)})}{(-T_o + T_s) \tau_{IIso}^2} & 1 \leq E < 2 \\ \frac{-e^{-\frac{1}{2}(T_o + T_s)(-1+E)} + e^{2T_o - T_s - T_o E}}{(T_o - T_s) \tau_{IIso}^2} & 2 \leq E < 3 \\ 0 & \text{else} \end{cases}$$

$$P_{18}(E | T_s = T_o) = \begin{cases} \frac{e^{T - T \cdot E}(E-1)}{2 \tau_{IIso}^2} & 1 \leq E < 2 \\ \frac{e^{T - T \cdot E}(3-E)}{2 \tau_{IIso}^2} & 2 \leq E < 3 \\ 0 & \text{else} \end{cases}$$

### Solution 19

**Description:** Electron (hole) creates a hole (electron). The electron (hole) creates an electron (hole).

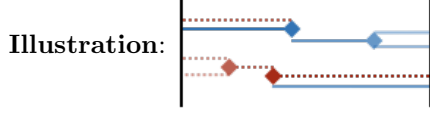

Combinatorial factor: 1

Solution:

$$P_{19}(E) = \begin{cases} -\frac{e^{T_o - T_s - T_o E} - e^{-2T_s + T_s E}}{T_o \tau_{IIso} \tau_{IIss} + T_s \tau_{IIso} \tau_{IIss}} & 1 \leq E < 2 \\ 0 & \text{else} \end{cases}$$

## Solution 20

**Description:** Electron (hole) creates a hole (electron). The electron (hole) traps. The hole (electron) creates a hole (electron).

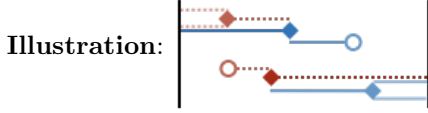

Combinatorial factor: 1

Solutions:

$$P_{20}(E | T_s \neq T_o) = \begin{cases} \frac{e^{-T_s E} \left( 3T_o - 3e^{\frac{2T_s E}{3}} T_o + T_s - 4e^{-\frac{1}{2}(T_o - T_s)E} T_s + 3e^{\frac{2T_s E}{3}} T_s \right)}{2\tau_{IIso} T_s (-3T_o^2 + 2T_o T_s + T_s^2) \tau_{IIso} \tau_{CTs}} & 0 \leq E < 1 \\ \frac{e^{-T_o E - \frac{1}{2}T_s(2+E)} (\zeta_1(E) + \zeta_2(E))}{2T_o \tau_{IIso} T_s (-T_o + T_s) (3T_o + T_s) \tau_{IIso} \tau_{CTs}} & 1 \leq E < 2 \\ -\frac{3e^{-T_s T_o} - 3e^{-\frac{T_s E}{3}} T_o + e^{-T_s T_s} - e^{-3T_o - T_s + T_o E} T_s}{6T_o^2 \tau_{IIso} T_s \tau_{CTs} + 2T_o \tau_{IIso} T_s^2 \tau_{IIso} \tau_{CTs}} & 2 \leq E < 3 \\ 0 & \text{else,} \end{cases}$$

where

$$\begin{aligned} \zeta_1(E) &= -4e^{T_s + \frac{T_o E}{2}} T_o T_s + 3e^{T_s + T_o E + \frac{T_s E}{6}} T_o (-T_o + T_s) \\ \zeta_2(E) &= e^{T_o + \frac{T_s E}{2}} T_s (3T_o + T_s) + e^{T_o E + \frac{T_s E}{2}} (3T_o^2 - 2T_o T_s - T_s^2) \end{aligned}$$

$$P_{20}(E | T_s = T_o) = \begin{cases} \frac{e^{-T \cdot E} \left( -3 + 3e^{\frac{2T \cdot E}{3}} - 2T \cdot E \right)}{8T^2 \tau_{IIso} \tau_{IIso} \tau_{CTs}} & 0 \leq E < 1 \\ \frac{e^{-T(5+2E)} \left( -4e^{2T(2+E)} + 3e^{\frac{5}{3}T(3+E)} + e^{T(5+E)} (1+2T(-2+E)) \right)}{8T^2 \tau_{IIso} \tau_{IIso} \tau_{CTs}} & 1 \leq E < 2 \\ -\frac{4e^{-T} - e^{T(-4+E)} - 3e^{-\frac{T \cdot E}{3}}}{8T^2 \tau_{IIso} \tau_{IIso} \tau_{CTs}} & 2 \leq E < 3 \\ 0 & \text{else} \end{cases}$$

## Solution 21

**Description:** Electron (hole) creates a hole (electron). The electron (hole) traps. The hole (electron) creates an electron (hole).

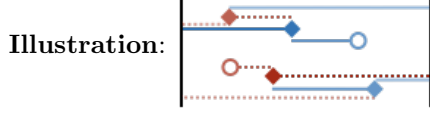

Combinatorial factor: 1

Solutions:

$$P_{21}(E | T_s \neq T_o) = \begin{cases} \frac{e^{\frac{1}{2}(T_o + T_s - T_o E - 3T_s E)} \zeta(E)}{\tau_{11os}(T_o - T_s)^2 \tau_{11so} \tau_{CTs}} & 1 \leq E < 2 \\ \frac{e^{\frac{1}{2}(T_o - 3T_o E - 3T_s(1+E))} \eta(E)}{\tau_{11os}(T_o - T_s)^2 \tau_{11so} \tau_{CTs}} & 2 \leq E < 3 \\ 0 & \text{else,} \end{cases}$$

where

$$\begin{aligned} \zeta(E) &= 2e^{T_s E} + e^{T_s + \frac{1}{2}(T_o + T_s)(-1+E)}(-2 + T_s + T_o(-1 + E) - T_s E) \\ \eta(E) &= 2e^{T_o E + T_s(2+E)} + e^{\frac{1}{2}(T_s + 3T_s E + T_o(3+E))}(-2 - T_o(-3 + E) + T_s(-3 + E)) \end{aligned}$$

$$P_{21}(E | T_s = T_o) = \begin{cases} \frac{e^{T - T \cdot E}(-1+E)^2}{4\tau_{11os} \tau_{11so} \tau_{CTs}} & 1 \leq E < 2 \\ \frac{e^{T - T \cdot E}(-3+E)^2}{4\tau_{11os} \tau_{11so} \tau_{CTs}} & 2 \leq E < 3 \\ 0 & \text{else} \end{cases}$$

## Solution 22

**Description:** Electron (hole) creates a hole (electron). The electron (hole) creates a hole (electron). The hole (electron) traps.

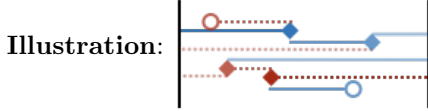

Combinatorial factor: 1

Solutions:

$$P_{22}(E | T_s \neq T_o) = \begin{cases} \frac{2e^{-\frac{1}{2}(T_o + T_s)(-1+E)} + e^{T_s - T_s E}(-2 + T_s + T_o(-1 + E) - T_s E)}{\tau_{CTo}(T_o - T_s)^2 \tau_{11so}^2} & 1 \leq E < 2 \\ \frac{e^{\frac{1}{2}(T_o - 2T_o E - T_s(2+E))} \left( 2e^{\frac{1}{2}(3T_s + T_o E)} + e^{\frac{1}{2}(3T_o + T_s E)}(-2 - T_o(-3 + E) + T_s(-3 + E)) \right)}{\tau_{CTo}(T_o - T_s)^2 \tau_{11so}^2} & 2 \leq E < 3 \\ 0 & \text{else} \end{cases}$$

$$P_{22}(E | T_s = T_o) = \begin{cases} \frac{e^{T - T \cdot E}(-1+E)^2}{4\tau_{CTo} \tau_{11so}^2} & 1 \leq E < 2 \\ \frac{e^{T - T \cdot E}(-3+E)^2}{4\tau_{CTo} \tau_{11so}^2} & 2 \leq E < 3 \\ 0 & \text{else} \end{cases}$$

### Solution 23

**Description:** Electron (hole) creates a hole (electron). The electron (hole) creates an electron (hole). The hole (electron) traps.

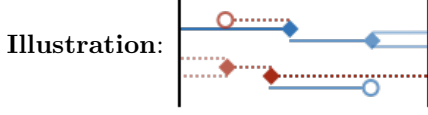

Combinatorial factor: 1

Solution:

$$P_{23}(E) = \begin{cases} \frac{e^{-2T_s - T_o E} (e^{T_o + T_s} - e^{(T_o + T_s)E}) (-2 + E)}{\tau_{CTo}(T_o + T_s) \tau_{IIsO} \tau_{IIsS}} & 1 \leq E < 2 \\ 0 & \text{else} \end{cases}$$

### Solution 24

**Description:** Electron (hole) creates a hole (electron). The electron (hole) creates an electron (hole). The hole (electron) creates an electron (hole).

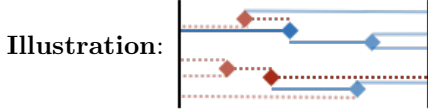

Combinatorial factor: 1

Solution:

$$P_{24}(E) = \begin{cases} \frac{e^{-3T_s - T_o E} (e^{2(T_o + T_s)} - e^{(T_o + T_s)E}) (-3 + E)}{\tau_{IIsO}(T_o + T_s) \tau_{IIsO} \tau_{IIsS}} & 2 \leq E < 3 \\ 0 & \text{else} \end{cases}$$

### Solution 25

**Description:** Electron (hole) creates a hole (electron). The electron (hole) creates an electron (hole). The hole (electron) creates a hole (electron).

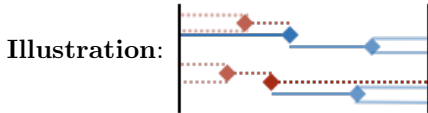

Combinatorial factor: 1

Solution:

$$P_{25}(E) = \begin{cases} \frac{e^{-2T_s - T_o E} (e^{(T_o + T_s)E} T_o + e^{T_o + T_s} T_s - e^{T_s + T_o E} (T_o + T_s))}{2T_o \tau_{IIsO} T_s (T_o + T_s) \tau_{IIsO} \tau_{IIsS}} & 1 \leq E < 2 \\ -\frac{e^{-T_s} (T_o - e^{-T_s(-3+E)} T_o + T_s - e^{T_o(-3+E)} T_s)}{2T_o \tau_{IIsO} T_s (T_o + T_s) \tau_{IIsO} \tau_{IIsS}} & 2 \leq E < 3 \\ 0 & \text{else} \end{cases}$$

### Solution 26

**Description:** Electron (hole) creates a hole (electron). The electron (hole) creates a hole (electron). The hole (electron) creates a hole (electron).

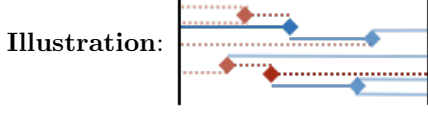

**Combinatorial factor:** 1

**Solutions:**

$$P_{26}(E | T_s \neq T_o) = \begin{cases} \frac{e^{\frac{T_s}{3} - \frac{T_o E}{2} - T_s E} \zeta(E)}{2\tau_{\text{Ilo}} T_s (-T_o + T_s) (3T_o + T_s) \tau_{\text{IIs}}^2} & 1 \leq E < 2 \\ \frac{e^{-T_o E - \frac{1}{2} T_s (2+E)} (\eta_1(E) + \eta_2(E))}{2T_o \tau_{\text{Ilo}} (T_o - T_s) T_s (3T_o + T_s) \tau_{\text{IIs}}^2} & 2 \leq E < 3 \\ -\frac{e^{-T_s} \left( \left( 3 - 3e^{-\frac{1}{3} T_s (-4+E)} \right) T_o + T_s - e^{T_o (-4+E)} T_s \right)}{2T_o \tau_{\text{Ilo}} T_s (3T_o + T_s) \tau_{\text{IIs}}^2} & 3 \leq E < 4 \\ 0 & \text{else} \end{cases}$$

where

$$\begin{aligned} \zeta(E) &= -3e^{\frac{1}{6} (3T_o + 4T_s) E} (T_o - T_s) - 4e^{\frac{1}{6} (3T_o + T_s + 3T_s E)} T_s + e^{\frac{2T_s}{3} + \frac{T_o E}{2}} (3T_o + T_s) \\ \eta_1(E) &= 3e^{T_o E + \frac{1}{6} T_s (8+E)} T_o (T_o - T_s) + 4e^{\frac{1}{2} (T_o + 3T_s + T_o E)} T_o T_s \\ \eta_2(E) &= -e^{2T_o + \frac{T_s E}{2}} T_s (3T_o + T_s) + e^{T_o E + \frac{T_s E}{2}} (-3T_o^2 + 2T_o T_s + T_s^2) \end{aligned}$$

$$P_{26}(E | T_s = T_o) = \begin{cases} \frac{3e^{\frac{1}{3} (T - T \cdot E)} + e^{T - T \cdot E} (-3 - 2T(-1+E))}{8T^2 \tau_{\text{Ilo}} \tau_{\text{IIs}}^2} & 1 \leq E < 2 \\ \frac{e^{-T(1+E)} (-4e^{T \cdot E} + 3e^{\frac{2}{3} T(2+E)} + e^{2T} (1 + 2T(-3+E)))}{8T^2 \tau_{\text{Ilo}} \tau_{\text{IIs}}^2} & 2 \leq E < 3 \\ -\frac{4e^{-T} - e^{T(-5+E)} - 3e^{\frac{1}{3} (T - T \cdot E)}}{8T^2 \tau_{\text{Ilo}} \tau_{\text{IIs}}^2} & 3 \leq E < 4 \\ 0 & \text{else} \end{cases}$$

### Solution 27

**Description:** Electron (hole) creates a hole (electron). The electron (hole) creates a hole (electron). The hole (electron) creates an electron (hole).

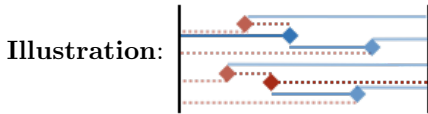

**Combinatorial factor:** 1

**Solutions:**

$$P_{27}(E | T_s \neq T_o) = \begin{cases} \frac{e^{-\frac{1}{2}(T_o+3T_s)(-2+E)} \left( 2e^{T_s(-2+E)} + e^{\frac{1}{2}(T_o+T_s)(-2+E)} (-2+T_o(-2+E)-T_s(-2+E)) \right)}{\tau_{\text{IIsos}}(T_o-T_s)^2 \tau_{\text{IIso}}^2} & 2 \leq E < 3 \\ \frac{e^{T_o - \frac{3T_o E}{2} - \frac{T_s E}{2}} \left( 2e^{T_s+T_o E} + e^{\frac{1}{2}(T_s(-2+E)+T_o(4+E))} (-2-T_o(-4+E)+T_s(-4+E)) \right)}{\tau_{\text{IIsos}}(T_o-T_s)^2 \tau_{\text{IIso}}^2} & 3 \leq E < 4 \\ 0 & \text{else} \end{cases}$$

$$P_{27}(E | T_s = T_o) = \begin{cases} \frac{e^{-T(-2+E)} (-2+E)^2}{4\tau_{\text{IIsos}} \tau_{\text{IIso}}^2} & 2 \leq E < 3 \\ \frac{e^{-T(-2+E)} (-4+E)^2}{4\tau_{\text{IIsos}} \tau_{\text{IIso}}^2} & 3 \leq E < 4 \\ 0 & \text{else} \end{cases}$$

### 3 Bulk-single-charge events

Bulk-single-charge events assume that the initial starting position of a charge (either  $e^-$  or  $h^+$ ) is randomly distributed throughout the bulk of the detector. The starting positions are taken to be a uniform distribution between the two surfaces. The general solutions for specific scenarios are the same whether the initial charge is an  $e^-$  or a  $h^+$ . What is only required is the distinction between parameters associated with the initial charge (parameters labelled with “s”) and parameters associated with the opposing charge (parameters labelled with “o”). The solutions for bulk-single-charge events are found up to second-order scenarios. That means that charges that participated or were produced in a primary II process can take part in no more than one additional II processes. Charges existing after the maximum number of II processes propagate to a crystal surface with 100% probability.

Each solution below provides a text description of the scenario, an illustration of the scenario, the combinatorial factor, and the unique analytical solution. In some cases, different solutions are required in the case where the  $T$  parameters are the same for electrons and holes. Also note that the combinatorial factor is already accounted for in the solutions provided.

The illustrations can be read as follows. The black, vertical bars represent the detector surfaces. Electrons are represented by blue, solid lines and propagate from left to right. Holes are represented by red, dashed lines and propagate from right to left. An open circle indicates that a charge is trapped, and a diamond indicates a charge has created another charge. The initial charge has the darkest shade, with charges existing after an occurrence of II having an increasingly lighter shade. The illustrations show both scenarios for when the initial charge is either an  $e^-$  or a  $h^+$ .

#### Solution 0

**Description:** Electron (hole) reaches the surface.

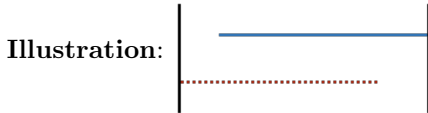

**Combinatorial factor:** 1

**Solution:**

$$P_0(E) = \begin{cases} e^{-T_s E} & 0 \leq E < 1 \\ 0 & \text{else} \end{cases}$$

### Solution 1

**Description:** Electron (hole) traps.

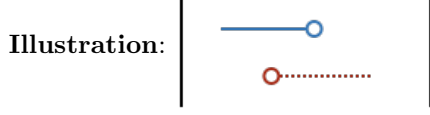

**Combinatorial factor:** 1

**Solution:**

$$P_1(E) = \begin{cases} \frac{e^{-T_s E}(1-E)}{\tau_{CTs}} & 0 \leq E < 1 \\ 0 & \text{else} \end{cases}$$

### Solution 2

**Description:** Electron (hole) creates an electron (hole).

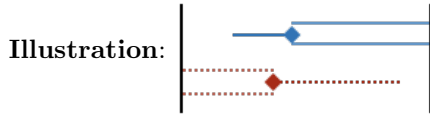

**Combinatorial factor:** 1

**Solution:**

$$P_2(E) = \begin{cases} \frac{e^{-T_s E} E}{2\tau_{IIs}} & 0 \leq E < 1 \\ \frac{e^{-T_s E}(2-E)}{2\tau_{IIs}} & 1 \leq E < 2 \\ 0 & \text{else} \end{cases}$$

### Solution 3

**Description:** Electron (hole) creates a hole (electron).

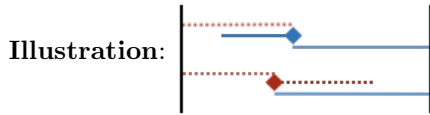

**Combinatorial factor:** 1

**Solutions:**

$$P_3(E | T_s \neq T_o) = \begin{cases} \frac{e^{T_o - T_s - T_o E} - e^{-T_o + T_s - T_s E}}{T_o \tau_{IIs} - T_s \tau_{IIs}} & 1 \leq E < 2 \\ 0 & \text{else} \end{cases}$$

$$P_3(E | T_s = T_o) = \begin{cases} \frac{e^{-T \cdot E}(2-E)}{\tau_{IIs}} & 1 \leq E < 2 \\ 0 & \text{else} \end{cases}$$

#### Solution 4

**Description:** Electron (hole) creates an electron (hole). One electron (hole) traps.

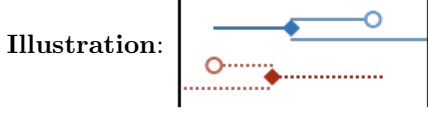

**Combinatorial factor:** 2

**Solution:**

$$P_4(E) = \begin{cases} \frac{e^{-T_s E} E^2}{2\tau_{\text{IIs}} \tau_{\text{CTs}}} & 0 \leq E < 1 \\ \frac{e^{-T_s E} (-2+E)^2}{2\tau_{\text{IIs}} \tau_{\text{CTs}}} & 1 \leq E < 2 \\ 0 & \text{else} \end{cases}$$

#### Solution 5

**Description:** Electron (hole) creates an electron (hole). Both electrons (holes) trap.

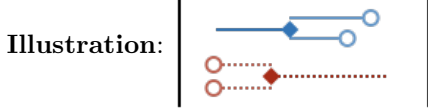

**Combinatorial factor:** 1

**Solution:**

$$P_5(E) = \begin{cases} \frac{e^{-T_s E} E^2 (6-5E)}{12\tau_{\text{IIs}} \tau_{\text{CTs}}^2} & 0 \leq E < 1 \\ \frac{e^{-T_s E} (2-E)^3}{12\tau_{\text{IIs}} \tau_{\text{CTs}}^2} & 1 \leq E < 2 \\ 0 & \text{else} \end{cases}$$

#### Solution 6

**Description:** Electron (hole) creates a hole (electron). The electron (hole) traps.

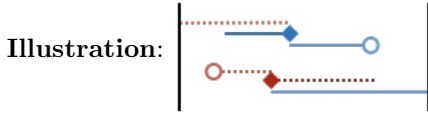

**Combinatorial factor:** 1

**Solutions:**

$$P_6(E | T_s \neq T_o) = \begin{cases} \frac{e^{-((T_o+T_s)E)} \left( e^{\frac{T_o E}{2}} - e^{\frac{T_s E}{2}} \right)^2}{(T_o - T_s)^2 \tau_{\text{IIs}} \tau_{\text{CTs}}} & 0 \leq E < 1 \\ \frac{e^{-((T_o+T_s)(1+E))} \left( e^{T_s + \frac{T_o E}{2}} - e^{T_o + \frac{T_s E}{2}} \right)^2}{(T_o - T_s)^2 \tau_{\text{IIs}} \tau_{\text{CTs}}} & 1 \leq E < 2 \\ 0 & \text{else} \end{cases}$$

$$P_6(E | T_s = T_o) = \begin{cases} \frac{e^{-T \cdot E} E^2}{4\tau_{\text{Iso}} \tau_{\text{CTs}}} & 0 \leq E < 1 \\ \frac{e^{-T \cdot E} (-2+E)^2}{4\tau_{\text{Iso}} \tau_{\text{CTs}}} & 1 \leq E < 2 \\ 0 & \text{else} \end{cases}$$

### Solution 7

**Description:** Electron (hole) creates a hole (electron). The hole (electron) traps.

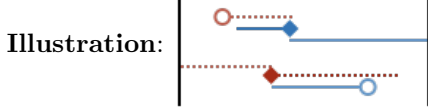

**Combinatorial factor:** 1

**Solutions:**

$$P_7(E | T_s \neq T_o) = \begin{cases} \frac{e^{-((T_o+T_s)E)} (e^{T_s E} + e^{T_o E} (-1+T_o E - T_s E))}{\tau_{\text{CTo}} (T_o - T_s)^2 \tau_{\text{Iso}}} & 0 \leq E < 1 \\ \frac{e^{-((T_o+T_s)(1+E))} (e^{2T_s+T_o E} + e^{2T_o+T_s E} (-1-T_o(-2+E) + T_s(-2+E)))}{\tau_{\text{CTo}} (T_o - T_s)^2 \tau_{\text{Iso}}} & 1 \leq E < 2 \\ 0 & \text{else} \end{cases}$$

$$P_7(E | T_s = T_o) = \begin{cases} \frac{e^{-T \cdot E} E^2}{2\tau_{\text{CTo}} \tau_{\text{Iso}}} & 0 \leq E < 1 \\ \frac{e^{-T \cdot E} (-2+E)^2}{2\tau_{\text{CTo}} \tau_{\text{Iso}}} & 1 \leq E < 2 \\ 0 & \text{else} \end{cases}$$

### Solution 8

**Description:** Electron (hole) creates a hole (electron). Both the electron and hole trap.

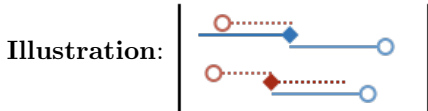

**Combinatorial factor:** 1

**Solutions:**

$$P_8(E | T_s \neq T_o) = \begin{cases} \frac{e^{-((T_o+T_s)E)} (4e^{\frac{1}{2}(T_o+T_s)E} + e^{T_s E} \zeta_1(E) + e^{T_o E} \zeta_2(E))}{\tau_{\text{CTo}} (T_o - T_s)^3 \tau_{\text{Iso}} \tau_{\text{CTs}}} & 0 \leq E < 1 \\ \frac{e^{-((T_o+T_s)(1+E))} (4e^{\frac{1}{2}(T_o+T_s)(2+E)} - e^{2T_s+T_o E} + e^{2T_o+T_s E} (-3-T_o(-2+E) + T_s(-2+E)))}{\tau_{\text{CTo}} (T_o - T_s)^3 \tau_{\text{Iso}} \tau_{\text{CTs}}} & 1 \leq E < 2 \\ 0 & \text{else,} \end{cases}$$

where

$$\zeta_1(E) = -1 + T_o + T_s(-1 + E) - T_o E$$

$$\zeta_2(E) = -3 + T_s - 2T_s E - T_o^2(-1 + E)E - T_s^2(-1 + E)E + T_o(-1 - 2(-1 + T_s)E + 2T_s E^2)$$

$$P_8(E | T_s = T_o) = \begin{cases} -\frac{e^{-T \cdot E} E^2 (-6+5E)}{12\tau_{CTo} \tau_{IIsO} \tau_{CTs}} & 0 \leq E < 1 \\ -\frac{e^{-T \cdot E} (-2+E)^3}{12\tau_{CTo} \tau_{IIsO} \tau_{CTs}} & 1 \leq E < 2 \\ 0 & \text{else} \end{cases}$$

### Solution 9

**Description:** Electron (hole) creates an electron (hole). One electron (hole) creates an electron (hole).

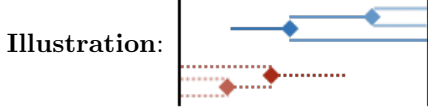

**Combinatorial factor:** 2

**Solution:**

$$P_9(E) = \begin{cases} \frac{e^{-T_s E} \left( -3 + 3e^{\frac{2T_s E}{3}} - 2T_s E \right)}{4T_s^2 \tau_{IIs}^2} & 0 \leq E < 1 \\ \frac{e^{-T_s E} \left( 1 + 3e^{\frac{2T_s E}{3}} - 4T_s + 2T_s E - 4e^{T_s E} \cosh[T_s] + 4e^{T_s E} \sinh[T_s] \right)}{4T_s^2 \tau_{IIs}^2} & 1 \leq E < 2 \\ -\frac{4e^{-T_s} - e^{T_s(-4+E)} - 3e^{-\frac{T_s E}{3}}}{4T_s^2 \tau_{IIs}^2} & 2 \leq E < 3 \\ 0 & \text{else} \end{cases}$$

### Solution 10

**Description:** Electron (hole) creates an electron (hole). One electron (hole) creates a hole (electron).

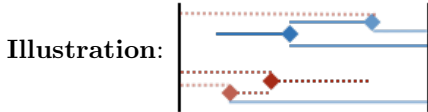

**Combinatorial factor:** 2

**Solution:**

$$P_{10}(E) = \begin{cases} \frac{e^{T_s - T_s E} (-1+E)^2}{2\tau_{IIsO} \tau_{IIs}} & 1 \leq E < 2 \\ \frac{e^{T_s - T_s E} (-3+E)^2}{2\tau_{IIsO} \tau_{IIs}} & 2 \leq E < 3 \\ 0 & \text{else} \end{cases}$$

### Solution 11

**Description:** Electron (hole) creates an electron (hole). One electron (hole) creates an electron (hole). The other electron (hole) traps.

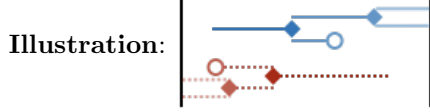

Combinatorial factor: 2

Solution:

$$P_{11}(E) = \begin{cases} \frac{e^{-T_s E} \left( 1 - 9e^{\frac{2T_s E}{3}} + 8e^{T_s E} - 2T_s E - 2T_s^2 E^2 \right)}{8T_s^3 \tau_{\text{IIs}}^2 \tau_{\text{CTs}}} & 0 \leq E < 1 \\ \frac{e^{-T_s E} \left( -1 + 8e^{T_s(-1+E)} - 9e^{\frac{2T_s E}{3}} + 8e^{T_s E} + e^{2T_s(-1+E)} \zeta_1(E) + \zeta_2(E) \right)}{8T_s^3 \tau_{\text{IIs}}^2 \tau_{\text{CTs}}} & 1 \leq E < 2 \\ \frac{-8e^{-T_s} + e^{T_s(-4+E)} - 2e^{-T_s(-2+E)} + 9e^{-\frac{T_s E}{3}}}{8T_s^3 \tau_{\text{IIs}}^2 \tau_{\text{CTs}}} & 2 \leq E < 3 \\ 0 & \text{else,} \end{cases}$$

where

$$\zeta_1(E) = -6 + 4T_s(-2 + E)$$

$$\zeta_2(E) = -2T_s(-2 + E) - 2T_s^2(-2 + E)^2$$

## Solution 12

**Description:** Electron (hole) creates an electron (hole). One electron (hole) creates a hole (electron). The other electron (hole) traps.

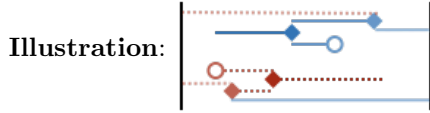

Combinatorial factor: 2

Solution:

$$P_{12}(E) = \begin{cases} -\frac{e^{T_s - T_s E} (-1+E)^2 (-11+5E)}{6\tau_{\text{IIs}} \tau_{\text{IIs}} \tau_{\text{CTs}}} & 1 \leq E < 2 \\ -\frac{e^{T_s - T_s E} (-3+E)^3}{6\tau_{\text{IIs}} \tau_{\text{IIs}} \tau_{\text{CTs}}} & 2 \leq E < 3 \\ 0 & \text{else} \end{cases}$$

## Solution 13

**Description:** Electron (hole) creates an electron (hole). Both electrons (holes) create an electron (hole).

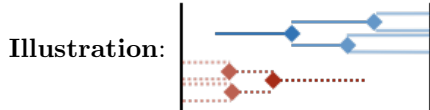

Combinatorial factor: 1

**Solution:**

$$P_{13}(E) = \begin{cases} \frac{e^{-T_s E} \left( 5 - 9e^{\frac{2T_s E}{3}} + 4e^{T_s E} + 2T_s E \right)}{16T_s^3 \tau_{\text{IIs}}^3} & 0 \leq E < 1 \\ \frac{e^{-T_s E} \left( -2 + 16e^{T_s(-1+E)} - 9e^{\frac{4}{3}T_s(-1+E)} - 9e^{\frac{2T_s E}{3}} + 4e^{T_s E} - 2T_s(-2+E) \right)}{16T_s^3 \tau_{\text{IIs}}^3} & 1 \leq E < 2 \\ \frac{e^{-\frac{1}{3}T_s(12+E)} \left( -9e^{4T_s} - 9e^{\frac{2}{3}T_s(4+E)} + 16e^{\frac{1}{3}T_s(9+E)} + 4e^{\frac{1}{3}T_s(12+E)} + 2e^{\frac{4T_s E}{3}}(-1+T_s(-2+E)) \right)}{16T_s^3 \tau_{\text{IIs}}^3} & 2 \leq E < 3 \\ \frac{4 - 9e^{\frac{1}{3}T_s(-4+E)} + e^{T_s(-4+E)}(5 - 2T_s(-4+E))}{16T_s^3 \tau_{\text{IIs}}^3} & 3 \leq E < 4 \\ 0 & \text{else} \end{cases}$$

### Solution 14

**Description:** Electron (hole) creates an electron (hole). Both electrons (holes) create a hole (electron).

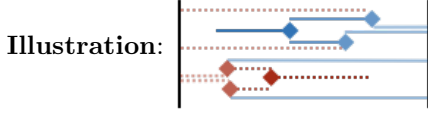

**Combinatorial factor:** 1

**Solution:**

$$P_{14}(E) = \begin{cases} -\frac{e^{-T_s(-2+E)}(-2+E)^2(-16+5E)}{12\tau_{\text{IIs}}^2 \tau_{\text{IIs}}} & 2 \leq E < 3 \\ -\frac{e^{-T_s(-2+E)}(-4+E)^3}{12\tau_{\text{IIs}}^2 \tau_{\text{IIs}}} & 3 \leq E < 4 \\ 0 & \text{else} \end{cases}$$

### Solution 15

**Description:** Electron (hole) creates an electron (hole). One electron (hole) creates an electron (hole). The other electron (hole) creates a hole (electron).

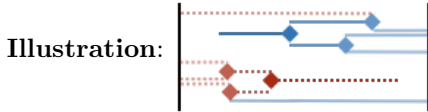

**Combinatorial factor:** 2

**Solution:**

$$P_{15}(E) = \begin{cases} \frac{e^{-T_s E} \left( 8e^{T_s E} - 9e^{\frac{1}{3}(T_s + 2T_s E)} + e^{T_s} (1 - 2T_s(-1+E) - 2T_s^2(-1+E)^2) \right)}{8T_s^3 \tau_{\text{IIs}} \tau_{\text{IIs}}^2} & 1 \leq E < 2 \\ \frac{e^{-T_s(3+2E)} \left( 8e^{2T_s(1+E)} - 9e^{\frac{5}{3}T_s(2+E)} + 8e^{T_s(3+2E)} + 2e^{3T_s E} \zeta_1(E) - e^{T_s(4+E)} \zeta_2(E) \right)}{8T_s^3 \tau_{\text{IIs}} \tau_{\text{IIs}}^2} & 2 \leq E < 3 \\ \frac{e^{-T_s(-3+E)} \left( 2 - 9e^{\frac{2}{3}T_s(-4+E)} + 8e^{T_s(-4+E)} - e^{2T_s(-4+E)} \right)}{8T_s^3 \tau_{\text{IIs}} \tau_{\text{IIs}}^2} & 3 \leq E < 4 \\ 0 & \text{else,} \end{cases}$$

where

$$\begin{aligned}\zeta_1(E) &= -3 + 2T_s(-3 + E) \\ \zeta_2(E) &= 1 + 2T_s(-3 + E) + 2T_s^2(-3 + E)^2\end{aligned}$$

### Solution 16

**Description:** Electron (hole) creates a hole (electron). The hole (electron) creates a hole (electron).

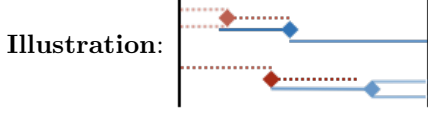

**Combinatorial factor:** 1

**Solutions:**

$$P_{16}(E | T_s \neq T_o) = \begin{cases} \frac{e^{-((T_o+T_s)(2+E))}(\zeta_1(E)+\zeta_2(E))}{2T_o\tau_{11oo}T_s(-T_o^2+T_s^2)\tau_{11so}} & 1 \leq E < 2 \\ -\frac{e^{-T_s}(T_o - e^{-T_s(-3+E)}T_o + T_s - e^{T_o(-3+E)}T_s)}{2T_o\tau_{11oo}T_s(T_o+T_s)\tau_{11so}} & 2 \leq E < 3 \\ 0 & \text{else,} \end{cases}$$

where

$$\begin{aligned}\zeta_1(E) &= -2e^{T_o+3T_s+T_oE}T_oT_s + 2e^{2T_oE+T_s(2+E)}T_oT_s - e^{2T_sE+T_o(2+E)}T_o(T_o+T_s) \\ \zeta_2(E) &= e^{3T_o+T_s+T_sE}T_s(T_o+T_s) + e^{2T_o+T_s+T_oE+T_sE}(T_o^2 - T_s^2)\end{aligned}$$

$$P_{16}(E | T_s = T_o) = \begin{cases} \frac{e^{-T(2+E)}(e^T - e^{T \cdot E})(e^{T \cdot E}(-1+2T(-2+E)) + e^T(1+2T(-2+E)))}{4T^2\tau_{11oo}\tau_{11so}} & 1 \leq E < 2 \\ \frac{e^{-T(-2+E)}(-1+e^{T(-3+E)})^2}{4T^2\tau_{11oo}\tau_{11so}} & 2 \leq E < 3 \\ 0 & \text{else} \end{cases}$$

### Solution 17

**Description:** Electron (hole) creates a hole (electron). The hole (electron) creates an electron (hole).

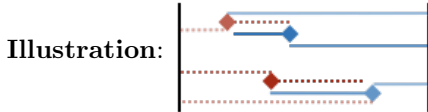

**Combinatorial factor:** 1

**Solutions:**

$$P_{17}(E | T_s \neq T_o) = \begin{cases} \frac{e^{T_o-T_oE}(1+e^{(T_o-T_s)(-1+E)}(-1+T_s+T_o(-1+E)-T_sE))}{\tau_{11os}(T_o-T_s)^2\tau_{11so}} & 1 \leq E < 2 \\ \frac{e^{-((T_o+T_s)(1+E))}(e^{3T_s+T_oE}+e^{3T_o+T_sE}(-1-T_o(-3+E)+T_s(-3+E)))}{\tau_{11os}(T_o-T_s)^2\tau_{11so}} & 2 \leq E < 3 \\ 0 & \text{else} \end{cases}$$

$$P_{17}(E | T_s = T_o) = \begin{cases} \frac{e^{T-T \cdot E}(-1+E)^2}{2\tau_{\text{IIsos}}\tau_{\text{IIso}}} & 1 \leq E < 2 \\ \frac{e^{T-T \cdot E}(-3+E)^2}{2\tau_{\text{IIsos}}\tau_{\text{IIso}}} & 2 \leq E < 3 \\ 0 & \text{else} \end{cases}$$

### Solution 18

**Description:** Electron (hole) creates a hole (electron). The electron (hole) creates a hole (electron).

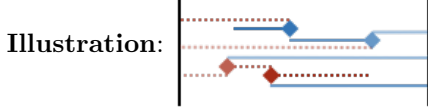

**Combinatorial factor:** 1

**Solutions:**

$$P_{18}(E | T_s \neq T_o) = \begin{cases} \frac{e^{-((T_o+T_s)E)} \left( -2e^{\frac{1}{2}(T_o+T_s)(1+E)} + e^{T_s+T_o E} + e^{T_o+T_s E} \right)}{(T_o-T_s)^2 \tau_{\text{IIso}}^2} & 1 \leq E < 2 \\ \frac{e^{-((T_o+T_s)(1+E))} \left( e^{\frac{1}{2}(3T_s+T_o E)} - e^{\frac{1}{2}(3T_o+T_s E)} \right)^2}{(T_o-T_s)^2 \tau_{\text{IIso}}^2} & 2 \leq E < 3 \\ 0 & \text{else} \end{cases}$$

$$P_{18}(E | T_s = T_o) = \begin{cases} \frac{e^{T-T \cdot E}(-1+E)^2}{4\tau_{\text{IIso}}^2} & 1 \leq E < 2 \\ \frac{e^{T-T \cdot E}(-3+E)^2}{4\tau_{\text{IIso}}^2} & 2 \leq E < 3 \\ 0 & \text{else} \end{cases}$$

### Solution 19

**Description:** Electron (hole) creates a hole (electron). The electron (hole) creates an electron (hole).

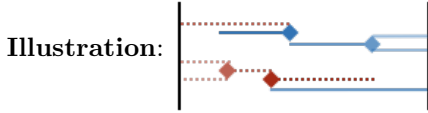

**Combinatorial factor:** 1

**Solutions:**

$$P_{19}(E | T_s = T_o) = \begin{cases} -\frac{e^{T_o(-2+E)} - e^{T_s(-2+E)} + e^{T_o-T_s-T_o E} - e^{-T_o+T_s-T_s E}}{(T_o^2-T_s^2)\tau_{\text{IIso}}\tau_{\text{IIss}}} & 1 \leq E < 2 \\ 0 & \text{else} \end{cases}$$

$$P_{19}(E | T_s = T_o) = \begin{cases} \frac{(-2+E)(\cosh[T] - \sinh[T]) \sinh[T-T \cdot E]}{T\tau_{\text{IIso}}\tau_{\text{IIss}}} & 1 \leq E < 2 \\ 0 & \text{else} \end{cases}$$

## Solution 20

**Description:** Electron (hole) creates a hole (electron). The electron (hole) traps. The hole (electron) creates a hole (electron).

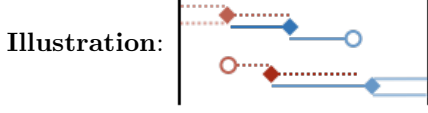

**Combinatorial factor:** 1

**Solutions:**

$$P_{20}(E | T_s \neq T_o) = \begin{cases} \frac{e^{-((T_o+T_s)E)}(\zeta_1(E)+\zeta_2(E)+\zeta_3(E))}{4T_o\tau_{I100}(T_o-T_s)^2T_s^2(3T_o+T_s)\tau_{I150}\tau_{CTs}} & 0 \leq E < 1 \\ \frac{e^{-4T_o(1+E)-\frac{1}{2}T_s(6+7E)}(\eta_1(E)+\eta_2(E)+\eta_3(E)+\eta_4(E)+\eta_5(E)+\eta_6(E))}{4T_o\tau_{I100}(T_o-T_s)^2T_s^2(T_o+T_s)(3T_o+T_s)\tau_{I150}\tau_{CTs}} & 1 \leq E < 2 \\ \frac{e^{-3T_o-T_s(1+E)}(\psi_1(E)+\psi_2(E))}{4T_o\tau_{I100}T_s^2(T_o+T_s)(3T_o+T_s)\tau_{I150}\tau_{CTs}} & 2 \leq E < 3 \\ 0 & \text{else,} \end{cases}$$

where

$$\begin{aligned} \zeta_1(E) &= -9e^{T_oE+\frac{2T_sE}{3}}T_o(T_o-T_s)^2+16e^{\frac{1}{2}(T_o+T_s)E}T_oT_s^2 \\ \zeta_2(E) &= 2e^{(T_o+T_s)E}(T_o-T_s)^2(3T_o+T_s)-2e^{T_sE}T_s^2(3T_o+T_s) \\ \zeta_3(E) &= e^{T_oE}T_o(3T_o^2-8T_oT_s-3T_s^2) \\ \eta_1(E) &= -9e^{4T_o(1+E)+T_s(3+\frac{19E}{6})}T_o(T_o-T_s)^2(T_o+T_s)+16e^{3T_s(1+E)+T_o(4+\frac{7E}{2})}T_oT_s^2(T_o+T_s) \\ \eta_2(E) &= -4e^{3T_o+4T_s+4T_oE+\frac{5T_sE}{2}}T_oT_s^2(3T_o+T_s)-2e^{2T_o+3T_s+5T_oE+\frac{7T_sE}{2}}T_s^2(-3T_o^2+2T_oT_s+T_s^2) \\ \eta_3(E) &= 2e^{4T_o+2T_s+4T_oE+\frac{7T_sE}{2}}(T_o-T_s)^2(3T_o^2+4T_oT_s+T_s^2) \\ \eta_4(E) &= 2e^{4T_o+3T_s+4T_oE+\frac{7T_sE}{2}}(T_o-T_s)^2(3T_o^2+4T_oT_s+T_s^2) \\ \eta_5(E) &= -2e^{5T_o+2T_s+3T_oE+\frac{7T_sE}{2}}T_s^2(3T_o^2+4T_oT_s+T_s^2) \\ \eta_6(E) &= e^{T_s+\frac{9T_sE}{2}+4T_o(1+E)}T_o(-3T_o^3-T_o^2T_s+3T_oT_s^2+T_s^3) \\ \psi_1(E) &= -2e^{(T_o+T_s)E}T_s^2-9e^{3T_o+T_s+\frac{2T_sE}{3}}T_o(T_o+T_s) \\ \psi_2(E) &= e^{3(T_o+T_s)}T_o(3T_o+T_s)+2e^{3T_o+T_sE}(3T_o^2+4T_oT_s+T_s^2) \end{aligned}$$

$$P_{20}(E | T_s = T_o) = \begin{cases} \frac{e^{-T \cdot E} \left( 1 - 9e^{\frac{2T \cdot E}{3}} + 8e^{T \cdot E} - 2T \cdot E - 2T^2 E^2 \right)}{16T^3\tau_{I100}\tau_{I150}\tau_{CTs}} & 0 \leq E < 1 \\ \frac{e^{-T(2+E)} \left( 8e^{T(2+E)} - 9e^{\frac{2}{3}T(3+E)} + 8e^{T+T \cdot E} + e^{2T \cdot E} \xi_1(E) - e^{2T} \xi_2(E) \right)}{16T^3\tau_{I100}\tau_{I150}\tau_{CTs}} & 1 \leq E < 2 \\ \frac{-8e^{-T} + e^{T(-4+E)} - 2e^{-T(-2+E)} + 9e^{-\frac{T \cdot E}{3}}}{16T^3\tau_{I100}\tau_{I150}\tau_{CTs}} & 2 \leq E < 3 \\ 0 & \text{else,} \end{cases}$$

where

$$\begin{aligned} \xi_1(E) &= -6 + 4T(-2 + E) \\ \xi_2(E) &= 1 + 2T(-2 + E) + 2T^2(-2 + E)^2 \end{aligned}$$

## Solution 21

**Description:** Electron (hole) creates a hole (electron). The electron (hole) traps. The hole (electron) creates an electron (hole).

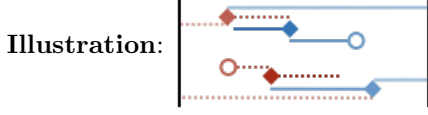

**Combinatorial factor:** 1

**Solutions:**

$$P_{21}(E | T_s \neq T_o) = \begin{cases} \frac{e^{-4T_o - 2T_s - 3T_o E - 4T_s E} \left( 4e^{\frac{1}{2}(T_o(9+5E) + T_s(5+7E))} + \zeta_1(E) - e^{3T_s(1+E) + T_o(4+3E)} \zeta_2(E) \right)}{\tau_{11os}(T_o - T_s)^3 \tau_{1iso} \tau_{CTs}} & 1 \leq E < 2 \\ \frac{e^{-((T_o + T_s)(1+E))} \left( 4e^{\frac{1}{2}(T_o + T_s)(3+E)} - e^{3T_s + T_o E} + e^{3T_o + T_s E} (-3 - T_o(-3+E) + T_s(-3+E)) \right)}{\tau_{11os}(T_o - T_s)^3 \tau_{1iso} \tau_{CTs}} & 2 \leq E < 3 \\ 0 & \text{else,} \end{cases}$$

where

$$\zeta_1(E) = e^{5T_o + 2T_s + 2T_o E + 4T_s E} (-1 - T_o(-2 + E) + T_s(-2 + E))$$

$$\zeta_2(E) = 3 + T_s(-3 + 2E) + T_o^2(2 - 3E + E^2) + T_s^2(2 - 3E + E^2) + T_o(3 - 2E - 2T_s(2 - 3E + E^2))$$

$$P_{21}(E | T_s = T_o) = \begin{cases} -\frac{e^{T-T \cdot E} (-1+E)^2 (-11+5E)}{12\tau_{11os} \tau_{1iso} \tau_{CTs}} & 1 \leq E < 2 \\ -\frac{e^{T-T \cdot E} (-3+E)^3}{12\tau_{11os} \tau_{1iso} \tau_{CTs}} & 2 \leq E < 3 \\ 0 & \text{else} \end{cases}$$

## Solution 22

**Description:** Electron (hole) creates a hole (electron). The electron (hole) creates a hole (electron). The hole (electron) traps.

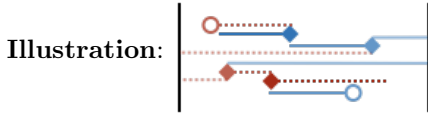

**Combinatorial factor:** 1

**Solutions:**

$$P_{22}(E | T_s \neq T_o) = \begin{cases} \frac{e^{-4T_o - 2T_s - \frac{7T_o E}{2} - 4T_s E} \left( 4e^{\frac{1}{2}(T_o(9+6E) + T_s(5+7E))} + \zeta_1(E) - e^{3T_s(1+E) + T_o(4+\frac{7E}{2})} \zeta_2(E) \right)}{\tau_{CTo}(T_o - T_s)^3 \tau_{1iso}^2} & 1 \leq E < 2 \\ \frac{e^{-((T_o + T_s)(1+E))} \left( 4e^{\frac{1}{2}(T_o + T_s)(3+E)} - e^{3T_s + T_o E} + e^{3T_o + T_s E} (-3 - T_o(-3+E) + T_s(-3+E)) \right)}{\tau_{CTo}(T_o - T_s)^3 \tau_{1iso}^2} & 2 \leq E < 3 \\ 0 & \text{else,} \end{cases}$$

where

$$\zeta_1(E) = e^{5T_o + 2T_s + \frac{5T_o E}{2} + 4T_s E} (-1 - T_o(-2 + E) + T_s(-2 + E))$$

$$\zeta_2(E) = 3 + T_s(-3 + 2E) + T_o^2(2 - 3E + E^2) + T_s^2(2 - 3E + E^2) + T_o(3 - 2E - 2T_s(2 - 3E + E^2))$$

$$P_{22}(E | T_s = T_o) = \begin{cases} -\frac{e^{T-T \cdot E}(-1+E)^2(-11+5E)}{12\tau_{CTo}\tau_{IIso}^2} & 1 \leq E < 2 \\ -\frac{e^{T-T \cdot E}(-3+E)^3}{12\tau_{CTo}\tau_{IIso}^2} & 2 \leq E < 3 \\ 0 & \text{else} \end{cases}$$

### Solution 23

**Description:** Electron (hole) creates a hole (electron). The electron (hole) creates an electron (hole). The hole (electron) traps.

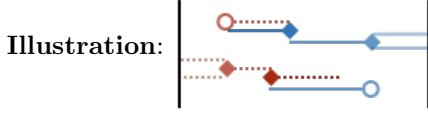

**Combinatorial factor:** 1

**Solutions:**

$$P_{23}(E | T_s \neq T_o) = \begin{cases} \frac{e^{-((T_o+T_s)E)}(e^{(T_o+T_s)E}(T_o-T_s)^2 - e^{T_s E}T_s^2 - e^{T_o E}T_o(T_o+T_oT_sE - T_s(2+T_sE))))}{2T_o\tau_{CTo}(T_o-T_s)^2T_s^2\tau_{IIso}\tau_{IIss}} & 0 \leq E < 1 \\ \frac{e^{-((T_o+T_s)(2+E))}(\zeta_1(E) + \zeta_2(E) + \zeta_3(E))}{2T_o\tau_{CTo}(T_o-T_s)^2T_s^2(T_o+T_s)\tau_{IIso}\tau_{IIss}} & 1 \leq E < 2 \\ 0 & \text{else,} \end{cases}$$

where

$$\begin{aligned} \zeta_1(E) &= -2e^{T_o+3T_s+T_oE}T_oT_s^2 + e^{2T_oE+T_s(2+E)}(T_o - T_s)T_s^2 \\ \zeta_2(E) &= e^{(T_o+T_s)(2+E)}(T_o - T_s)^2(T_o + T_s) + 2e^{3T_o+T_s+T_sE}T_oT_s^2(1 + T_o(-2 + E) - T_s(-2 + E)) \\ \zeta_3(E) &= e^{2T_sE+T_o(2+E)}T_o(-T_o + T_s)(T_o - T_oT_s(-2 + E) + T_s^2(-2 + E)) \end{aligned}$$

$$P_{23}(E | T_s = T_o) = \begin{cases} \frac{e^{-T \cdot E}(-2+2e^{T \cdot E}-2T \cdot E-T^2E^2)}{4T^3\tau_{CTo}\tau_{IIso}\tau_{IIss}} & 0 \leq E < 1 \\ \frac{e^{-2T(1+E)}(2e^{2T(1+E)}+2e^{3T \cdot E}(-1+T(-2+E))-e^{T(2+E)}T^2(-2+E)^2)}{4T^3\tau_{CTo}\tau_{IIso}\tau_{IIss}} & 1 \leq E < 2 \\ 0 & \text{else} \end{cases}$$

### Solution 24

**Description:** Electron (hole) creates a hole (electron). The electron (hole) creates an electron (hole). The hole (electron) creates an electron (hole).

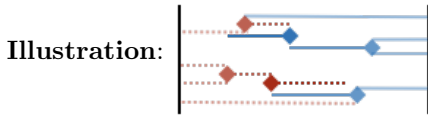

**Combinatorial factor:** 1

**Solutions:**

$$P_{24}(E | T_s \neq T_o) = \begin{cases} \frac{(T_o - T_s)^2 - e^{T_o - T_o E} T_s^2 - e^{T_s - T_s E} T_o (T_o + T_o T_s (-1 + E) + T_s (-2 + T_s - T_s E))}{2 T_o \tau_{IIos} (T_o - T_s)^2 T_s^2 \tau_{IIso} \tau_{IIss}} & 1 \leq E < 2 \\ \frac{e^{-((T_o + T_s)(3 + E))} (\zeta_1(E) + \zeta_2(E) + \zeta_3(E))}{2 T_o \tau_{IIos} (T_o - T_s)^2 T_s^2 (T_o + T_s) \tau_{IIso} \tau_{IIss}} & 2 \leq E < 3 \\ 0 & \text{else,} \end{cases}$$

where

$$\begin{aligned} \zeta_1(E) &= -2e^{5T_s + T_o(2 + E)} T_o T_s^2 + e^{2T_o E + T_s(3 + E)} (T_o - T_s) T_s^2 \\ \zeta_2(E) &= e^{(T_o + T_s)(3 + E)} (T_o - T_s)^2 (T_o + T_s) + 2e^{5T_o + T_s(2 + E)} T_o T_s^2 (1 + T_o(-3 + E) - T_s(-3 + E)) \\ \zeta_3(E) &= e^{2T_s E + T_o(3 + E)} T_o (-T_o + T_s) (T_o - T_o T_s(-3 + E) + T_s^2(-3 + E)) \end{aligned}$$

$$P_{24}(E | T_s = T_o) = \begin{cases} \frac{e^{-T \cdot E} (4e^{T \cdot E} - 2e^T (2 + 2T(-1 + E) + T^2(-1 + E)^2))}{8T^3 \tau_{IIos} \tau_{IIso} \tau_{IIss}} & 1 \leq E < 2 \\ \frac{e^{-T \cdot E} (2e^{T \cdot E} + 2e^{T(-3 + 2E)} (-1 + T(-3 + E)) - e^T T^2(-3 + E)^2)}{4T^3 \tau_{IIos} \tau_{IIso} \tau_{IIss}} & 2 \leq E < 3 \\ 0 & \text{else} \end{cases}$$

## Solution 25

**Description:** Electron (hole) creates a hole (electron). The electron (hole) creates an electron (hole). The hole (electron) creates a hole (electron).

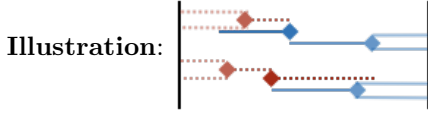

**Combinatorial factor:** 1

**Solutions:**

$$P_{25}(E | T_s \neq T_o) = \begin{cases} \frac{e^{-((T_o + T_s)(2 + E))} (\zeta_1(E) + \zeta_2(E) + \zeta_3(E))}{2 T_o \tau_{IIoo} (T_o - T_s) T_s^2 (T_o + T_s)^2 \tau_{IIso} \tau_{IIss}} & 1 \leq E < 2 \\ \frac{e^{-3T_o - T_s(1 + E)} (\eta_1(E) + \eta_2(E))}{2 T_o \tau_{IIoo} T_s^2 (T_o + T_s)^2 \tau_{IIso} \tau_{IIss}} & 2 \leq E < 3 \\ 0 & \text{else,} \end{cases}$$

where

$$\begin{aligned} \zeta_1(E) &= -2e^{T_o + 3T_s + T_o E} T_o T_s^2 + e^{3T_o + T_s + T_s E} T_s^2 (T_o + T_s) \\ \zeta_2(E) &= e^{2T_o + T_s + T_o E + T_s E} (T_o - T_s) (T_o + T_s)^2 - 2e^{2T_o E + T_s(2 + E)} T_o T_s^2 (-1 + T_o(-1 + E) + T_s(-1 + E)) \\ \zeta_3(E) &= e^{2T_s E + T_o(2 + E)} T_o (T_o + T_s) (T_o(-1 + T_s(-1 + E)) + T_s^2(-1 + E)) \\ \eta_1(E) &= -e^{(T_o + T_s)E} T_s^2 + e^{3T_o + T_s E} (T_o + T_s)^2 \\ \eta_3(E) &= -e^{3(T_o + T_s)} T_o (T_o + T_s(2 + T_s(-3 + E)) + T_o T_s(-3 + E)) \end{aligned}$$

$$P_{25}(E | T_s = T_o) = \begin{cases} \frac{e^{-T(2 + E)} (4e^{T + T \cdot E} + e^{2T} (-1 - 2T(-2 + E)) - e^{2T \cdot E} (3 + T(6 - 4E) + 4T^2(2 - 3E + E^2)))}{8T^3 \tau_{IIoo} \tau_{IIso} \tau_{IIss}} & 1 \leq E < 2 \\ \frac{e^{-T(4 + E)} (-e^{2T \cdot E} + 4e^{T(3 + E)} + e^{6T} (-3 - 2T(-3 + E)))}{8T^3 \tau_{IIoo} \tau_{IIso} \tau_{IIss}} & 2 \leq E < 3 \\ 0 & \text{else} \end{cases}$$

## Solution 26

**Description:** Electron (hole) creates a hole (electron). The electron (hole) creates a hole (electron). The hole (electron) creates a hole (electron).

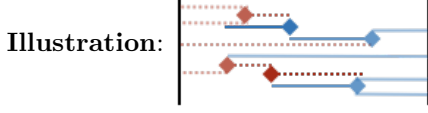

**Combinatorial factor:** 1

**Solutions:**

$$P_{26}(E | T_s \neq T_o) = \begin{cases} \frac{e^{-\frac{23T_o E}{4} - T_s E} (\zeta_1(E) + \zeta_2(E) + \zeta_3(E))}{4T_o \tau_{\text{Ilo}} (T_o - T_s)^2 T_s^2 (3T_o + T_s) \tau_{\text{Iso}}^2} & 1 \leq E < 2 \\ \frac{e^{-\frac{7}{2}T_o(1+3E) - T_s(5+6E)} (\eta_1(E) + \eta_2(E) + \eta_3(E) + \eta_4(E) + \eta_5(E) + \eta_6(E))}{4T_o \tau_{\text{Ilo}} (T_o - T_s)^2 T_s^2 (T_o + T_s) (3T_o + T_s) \tau_{\text{Iso}}^2} & 2 \leq E < 3 \\ \frac{e^{-2T_s(-1+E)} (\psi_1(E) + \psi_2(E))}{4T_o \tau_{\text{Ilo}} T_s^2 (T_o + T_s) (3T_o + T_s) \tau_{\text{Iso}}^2} & 3 \leq E < 4 \\ 0 & \text{else,} \end{cases}$$

where

$$\begin{aligned} \zeta_1(E) &= -9e^{\frac{1}{12}(69T_o E + T_s(4+8E))} T_o (T_o - T_s)^2 + 16e^{\frac{1}{4}(2T_s(1+E) + T_o(2+21E))} T_o T_s^2 \\ \zeta_2(E) &= 2e^{\frac{23T_o E}{4} + T_s E} (T_o - T_s)^2 (3T_o + T_s) - 2e^{T_o + \frac{19T_o E}{4} + T_s E} T_s^2 (3T_o + T_s) \\ \zeta_3(E) &= e^{T_s + \frac{23T_o E}{4}} T_o (3T_o^2 - 8T_o T_s - 3T_s^2) \\ \eta_1(E) &= -9e^{\frac{1}{6}(21T_o + 32T_s + 63T_o E + 34T_s E)} T_o (T_o - T_s)^2 (T_o + T_s) + 16e^{\frac{11}{2}T_s(1+E) + 2T_o(2+5E)} T_o T_s^2 (T_o + T_s) \\ \eta_2(E) &= -4e^{T_s(7+5E) + \frac{1}{2}T_o(5+21E)} T_o T_s^2 (3T_o + T_s) - 2e^{\frac{1}{2}(T_o + 23T_o E + 2T_s(5+6E))} T_s^2 (-3T_o^2 + 2T_o T_s + T_s^2) \\ \eta_3(E) &= 2e^{\frac{7}{2}T_o(1+3E) + 2T_s(2+3E)} (T_o - T_s)^2 (3T_o^2 + 4T_o T_s + T_s^2) \\ \eta_4(E) &= 2e^{\frac{7}{2}T_o(1+3E) + T_s(5+6E)} (T_o - T_s)^2 (3T_o^2 + 4T_o T_s + T_s^2) \\ \eta_5(E) &= -2e^{\frac{11T_o}{2} + 4T_s + \frac{19T_o E}{2} + 6T_s E} T_s^2 (3T_o^2 + 4T_o T_s + T_s^2) \\ \eta_6(E) &= -e^{\frac{7}{2}T_o(1+3E) + T_s(2+7E)} T_o (3T_o^3 + T_o^2 T_s - 3T_o T_s^2 - T_s^3) \\ \psi_1(E) &= -2e^{T_s + (T_o + T_s)(-4+E) + T_s E} T_s^2 - 9e^{\frac{5}{3}T_s(-1+E)} T_o (T_o + T_s) \\ \psi_2(E) &= e^{T_s + T_s E} T_o (3T_o + T_s) + 2e^{T_s(-3+2E)} (3T_o^2 + 4T_o T_s + T_s^2) \end{aligned}$$

$$P_{26}(E | T_s = T_o) = \begin{cases} \frac{e^{-T \cdot E} \left( 8e^{T \cdot E} - 9e^{\frac{1}{3}(T + 2T \cdot E)} + e^T (1 - 2T(-1+E) - 2T^2(-1+E)^2) \right)}{16T^3 \tau_{\text{Ilo}} \tau_{\text{Iso}}^2} & 1 \leq E < 2 \\ \frac{e^{-3T(5+E)} (\xi_1(E) + \xi_2(E))}{16T^3 \tau_{\text{Ilo}} \tau_{\text{Iso}}^2} & 2 \leq E < 3 \\ \frac{e^{-T(-3+E)} \left( 2 - 9e^{\frac{2}{3}T(-4+E)} + 8e^{T(-4+E)} - e^{2T(-4+E)} \right)}{16T^3 \tau_{\text{Ilo}} \tau_{\text{Iso}}^2} & 3 \leq E < 4 \\ 0 & \text{else,} \end{cases}$$

where

$$\begin{aligned} \xi_1(E) &= 7e^{3T(5+E)} + 8e^{T(14+3E)} - 9e^{\frac{2}{3}T(23+4E)} + e^{T(9+5E)} + 2e^{4T(3+E)} (-3 + 2T(-3 + E)) \\ \xi_2(E) &= -e^{2T(8+E)} (1 + 2T(-3 + E) + 2T^2(-3 + E)^2) + 2e^{4T(3+E)} \sinh[3T - T \cdot E] \end{aligned}$$

## Solution 27

**Description:** Electron (hole) creates a hole (electron). The electron (hole) creates a hole (electron). The hole (electron) creates an electron (hole).

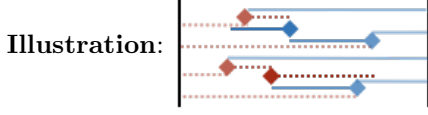

**Combinatorial factor:** 1

**Solutions:**

$$P_{27}(E | T_s \neq T_o) = \begin{cases} \frac{e^{-2(T_o+T_s)(-1+E)} (\zeta_1(E) - e^{2T_o(-1+E)+T_s E} \zeta_2(E))}{\tau_{\text{Hos}}(T_o - T_s)^3 \tau_{\text{Iso}}^2} & 2 \leq E < 3 \\ \frac{e^{T_o - T_o E - T_s(1+E)} (-e^{4T_s+T_o(-2+E)} + 4e^{\frac{1}{2}(T_o E + T_s(4+E))} + e^{2T_o+T_s E} \eta(E))}{\tau_{\text{Hos}}(T_o - T_s)^3 \tau_{\text{Iso}}^2} & 3 \leq E < 4 \\ 0 & \text{else,} \end{cases}$$

where

$$\begin{aligned} \zeta_1(E) &= 4e^{\frac{1}{2}(T_o+T_s)(-2+3E)} + e^{2T_s(-1+E)+T_o E} (-1 - T_o(-3+E) + T_s(-3+E)) \\ \zeta_2(E) &= 3 + T_s(-5+2E) + T_o^2(6-5E+E^2) + T_s^2(6-5E+E^2) + T_o(5-2E-2T_s(6-5E+E^2)) \\ \eta(E) &= -3 - T_o(-4+E) + T_s(-4+E) \end{aligned}$$

$$P_{27}(E | T_s = T_o) = \begin{cases} -\frac{e^{-T(-2+E)}(-2+E)^2(-16+5E)}{12\tau_{\text{Hos}}\tau_{\text{Iso}}^2} & 2 \leq E < 3 \\ -\frac{e^{-T(-2+E)}(-4+E)^3}{12\tau_{\text{Hos}}\tau_{\text{Iso}}^2} & 3 \leq E < 4 \\ 0 & \text{else} \end{cases}$$

## 4 Bulk- $e^-h^+$ -pair events

Bulk- $e^-h^+$ -pair events assume that the initial starting position of an  $e^-h^+$  pair is randomly distributed throughout the bulk of the detector. The starting positions are taken to be a uniform distribution between the two surfaces. The solutions for bulk- $e^-h^+$ -pair events are found up to first-order scenarios. That means that charges that participated or were produced in a primary II process propagate to a crystal surface with 100% probability.

Each solution below provides a text description of the scenario, an illustration of the scenario, and the unique analytical solution. Different solutions are required in the case where the  $T$  parameters are the same for electrons and holes. The illustrations can be read as follows. The black, vertical bars represent the detector surfaces. Electrons are represented by blue, solid lines and propagate from left to right. Holes are represented by red, dashed lines and propagate from right to left. An open circle indicates that a charge is trapped, and a diamond indicates a charge has created another charge. The initial charges have the darkest shade, with charges existing after an occurrence of II having an increasingly lighter shade.

### Solution 0

**Description:** Both the electron and hole reach the surface.

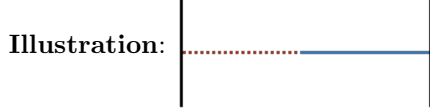

Solutions:

$$P_0(E | T_e \neq T_h) = \delta(E - 1) \frac{e^{-T_e} - e^{-T_h}}{T_h - T_e}$$

$$P_0(E | T_e = T_h) = \delta(E - 1) e^{-T}$$

### Solution 1

**Description:** The electron traps and the hole reaches the surface.

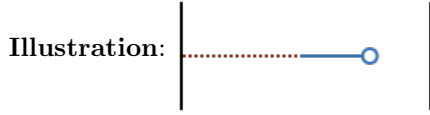

Solutions:

$$P_1(E | T_e \neq T_h) = \begin{cases} -\frac{e^{-T_e E} - e^{-T_h E}}{T_e \tau_{CTe} - \tau_{CTe} T_h} & 0 \leq E < 1 \\ 0 & \text{else} \end{cases}$$

$$P_1(E | T_e = T_h) = \begin{cases} \frac{e^{-T \cdot E}}{\tau_{CTe}} & 0 \leq E < 1 \\ 0 & \text{else} \end{cases}$$

### Solution 2

**Description:** The electron creates an electron and the hole reaches the surface.

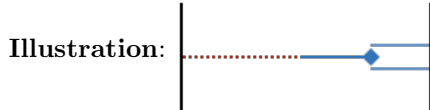

Solutions:

$$P_2(E | T_e \neq T_h) = \begin{cases} -\frac{e^{T_e(-2+E)} + e^{T_h(-2+E)}}{\tau_{11ee}(T_e - T_h)} & 1 \leq E < 2 \\ 0 & \text{else} \end{cases}$$

$$P_2(E | T_e = T_h) = \begin{cases} -\frac{e^{T(-2+E)}(-2+E)}{\tau_{11ee}} & 1 \leq E < 2 \\ 0 & \text{else} \end{cases}$$

### Solution 3

**Description:** The electron creates a hole and the hole reaches the surface.

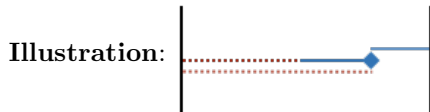

**Solutions:**

$$P_3(E | T_e \neq T_h) = \begin{cases} -\frac{e^{-T_e - T_e E} - e^{-T_h - T_h E}}{T_e \tau_{11eh} - \tau_{11eh} T_h} & 1 \leq E < 2 \\ 0 & \text{else} \end{cases}$$

$$P_3(E | T_e = T_h) = \begin{cases} \frac{e^{-T \cdot E} (-1+E)}{\tau_{11eh}} & 1 \leq E < 2 \\ 0 & \text{else} \end{cases}$$

#### Solution 4

**Description:** The electron reaches the surface and the hole traps.

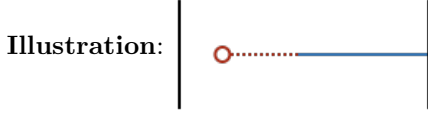

**Solutions:**

$$P_4(E | T_e \neq T_h) = \begin{cases} -\frac{e^{-T_e E} - e^{-T_h E}}{T_e \tau_{CTh} - T_h \tau_{CTh}} & 0 \leq E < 1 \\ 0 & \text{else} \end{cases}$$

$$P_4(E | T_e = T_h) = \begin{cases} \frac{e^{-T \cdot E}}{\tau_{CTh}} & 0 \leq E < 1 \\ 0 & \text{else} \end{cases}$$

#### Solution 5

**Description:** The electron traps and the hole traps.

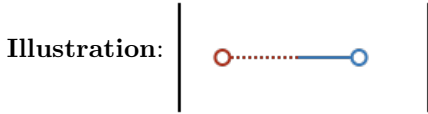

**Solutions:**

$$P_5(E | T_e \neq T_h) = \begin{cases} \frac{e^{-((T_e + T_h)E)} (-e^{T_e E} + e^{T_h E}) (-1+E)}{\tau_{CTe} (T_e - T_h) \tau_{CTh}} & 0 \leq E < 1 \\ 0 & \text{else} \end{cases}$$

$$P_5(E | T_e = T_h) = \begin{cases} -\frac{e^{-T \cdot E} (-1+E)E}{\tau_{CTe} \tau_{CTh}} & 0 \leq E < 1 \\ 0 & \text{else} \end{cases}$$

#### Solution 6

**Description:** The electron creates an electron and the hole traps.

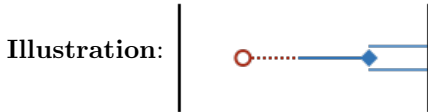

**Solutions:**

$$P_6(E | T_e \neq T_h) = \begin{cases} \frac{T_e - e^{-T_h E} T_e - T_h + e^{-T_e E} T_h}{2T_e^2 \tau_{Ilee} T_h \tau_{CTh} - 2T_e \tau_{Ilee} T_h^2 \tau_{CTh}} & 0 \leq E < 1 \\ \frac{T_e - e^{-2T_h + T_h E} T_e - T_h + e^{-2T_e + T_e E} T_h}{2T_e^2 \tau_{Ilee} T_h \tau_{CTh} - 2T_e \tau_{Ilee} T_h^2 \tau_{CTh}} & 1 \leq E < 2 \\ 0 & \text{else} \end{cases}$$

$$P_6(E | T_e = T_h) = \begin{cases} \frac{e^{-T \cdot E} (-1 + e^{T \cdot E} - T \cdot E)}{2T^2 \tau_{Ilee} \tau_{CTh}} & 0 \leq E < 1 \\ \frac{1 + e^{T(-2+E)} (-1 + T(-2+E))}{2T^2 \tau_{Ilee} \tau_{CTh}} & 1 \leq E < 2 \\ 0 & \text{else} \end{cases}$$

### Solution 7

**Description:** The electron creates a hole and the hole traps.

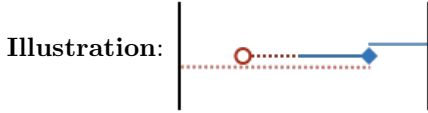

**Solutions:**

$$P_7(E | T_e \neq T_h) = \begin{cases} -\frac{e^{-((T_e+T_h)E)} (e^{T_h+T_e E} - e^{T_e+T_h E}) (-2+E)}{\tau_{Ileh} (T_e - T_h) \tau_{CTh}} & 1 \leq E < 2 \\ 0 & \text{else} \end{cases}$$

$$P_7(E | T_e = T_h) = \begin{cases} -\frac{e^{T-T \cdot E} (2-3E+E^2)}{\tau_{Ileh} \tau_{CTh}} & 1 \leq E < 2 \\ 0 & \text{else} \end{cases}$$

### Solution 8

**Description:** The electron reaches the surface and the hole creates a hole.

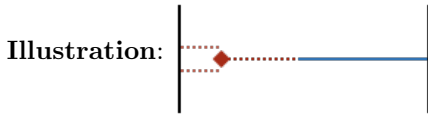

**Solutions:**

$$P_8(E | T_e \neq T_h) = \begin{cases} \frac{-e^{T_e(-2+E)} + e^{T_h(-2+E)}}{(T_e - T_h) \tau_{IIhh}} & 1 \leq E < 2 \\ 0 & \text{else} \end{cases}$$

$$P_8(E | T_e = T_h) = \begin{cases} -\frac{e^{T(-2+E)} (-2+E)}{\tau_{IIhh}} & 1 \leq E < 2 \\ 0 & \text{else} \end{cases}$$

### Solution 9

**Description:** The electron traps and the hole creates a hole.

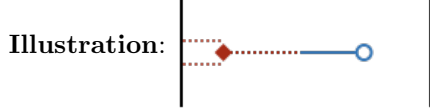

Solutions:

$$P_9(E | T_e \neq T_h) = \begin{cases} \frac{T_e - e^{-T_h E} T_e - T_h + e^{-T_e E} T_h}{2T_e^2 \tau_{CTe} T_h \tau_{Ihh} - 2T_e \tau_{CTe} T_h^2 \tau_{Ihh}} & 0 \leq E < 1 \\ \frac{T_e - e^{-2T_h + T_h E} T_e - T_h + e^{-2T_e + T_e E} T_h}{2T_e^2 \tau_{CTe} T_h \tau_{Ihh} - 2T_e \tau_{CTe} T_h^2 \tau_{Ihh}} & 1 \leq E < 2 \\ 0 & \text{else} \end{cases}$$

$$P_9(E | T_e = T_h) = \begin{cases} \frac{e^{-T \cdot E} (-1 + e^{T \cdot E} - T \cdot E)}{2T^2 \tau_{CTe} \tau_{Ihh}} & 0 \leq E < 1 \\ \frac{1 + e^{T(-2+E)} (-1 + T(-2+E))}{2T^2 \tau_{CTe} \tau_{Ihh}} & 1 \leq E < 2 \\ 0 & \text{else} \end{cases}$$

### Solution 10

**Description:** The electron creates an electron and the hole creates a hole.

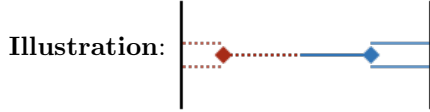

Solutions:

$$P_{10}(E | T_e \neq T_h) = \begin{cases} -\frac{(e^{T_e(-2+E)} - e^{T_h(-2+E)})(-1+E)}{\tau_{Iee}(T_e - T_h) \tau_{Ihh}} & 1 \leq E < 2 \\ 0 & \text{else} \end{cases}$$

$$P_{10}(E | T_e = T_h) = \begin{cases} -\frac{e^{T(-2+E)} (2-3E+E^2)}{\tau_{Iee} \tau_{Ihh}} & 1 \leq E < 2 \\ 0 & \text{else} \end{cases}$$

### Solution 11

**Description:** The electron creates a hole and the hole creates a hole.

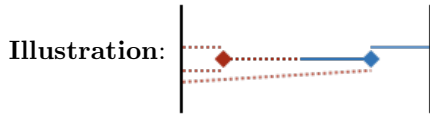

Solutions:

$$P_{11}(E | T_e \neq T_h) = \begin{cases} \frac{T_e - e^{T_h - T_h E} T_e - T_h + e^{T_e - T_e E} T_h}{2T_e^2 \tau_{Ieh} T_h \tau_{Ihh} - 2T_e \tau_{Ieh} T_h^2 \tau_{Ihh}} & 1 \leq E < 2 \\ \frac{T_e - e^{-3T_h + T_h E} T_e - T_h + e^{-3T_e + T_e E} T_h}{2T_e^2 \tau_{Ieh} T_h \tau_{Ihh} - 2T_e \tau_{Ieh} T_h^2 \tau_{Ihh}} & 2 \leq E < 3 \\ 0 & \text{else} \end{cases}$$

$$P_{11}(E | T_e = T_h) = \begin{cases} \frac{e^{-T \cdot E} (e^{T \cdot E} + e^T (-1 + T - T \cdot E))}{2T^2 \tau_{I1eh} \tau_{I1hh}} & 1 \leq E < 2 \\ \frac{1 + e^{T(-3+E)} (-1 + T(-3+E))}{2T^2 \tau_{I1eh} \tau_{I1hh}} & 2 \leq E < 3 \\ 0 & \text{else} \end{cases}$$

### Solution 12

**Description:** The electron reaches the surface and the hole creates an electron.

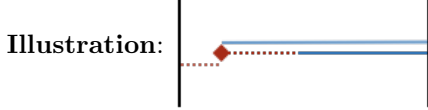

**Solutions:**

$$P_{12}(E | T_e \neq T_h) = \begin{cases} -\frac{e^{T_e - T_h E} - e^{T_h - T_h E}}{T_e \tau_{I1he} - T_h \tau_{I1he}} & 1 \leq E < 2 \\ 0 & \text{else} \end{cases}$$

$$P_{12}(E | T_e = T_h) = \begin{cases} \frac{e^{T - T \cdot E} (-1 + E)}{\tau_{I1he}} & 1 \leq E < 2 \\ 0 & \text{else} \end{cases}$$

### Solution 13

**Description:** The electron traps and the hole creates an electron.

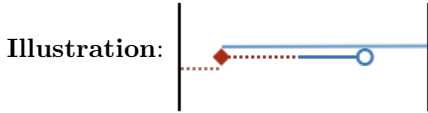

**Solutions:**

$$P_{13}(E | T_e \neq T_h) = \begin{cases} -\frac{e^{-((T_e + T_h)E)} (e^{T_h + T_e E} - e^{T_e + T_h E}) (-2 + E)}{\tau_{CTe} (T_e - T_h) \tau_{I1he}} & 1 \leq E < 2 \\ 0 & \text{else} \end{cases}$$

$$P_{13}(E | T_e = T_h) = \begin{cases} -\frac{e^{T - T \cdot E} (2 - 3E + E^2)}{\tau_{CTe} \tau_{I1he}} & 1 \leq E < 2 \\ 0 & \text{else} \end{cases}$$

### Solution 14

**Description:** The electron creates an electron and the hole creates an electron.

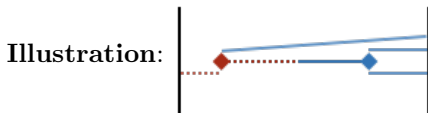

**Solutions:**

$$P_{14}(E | T_e \neq T_h) = \begin{cases} \frac{T_e - e^{T_h - T_h E} T_e - T_h + e^{T_e - T_e E} T_h}{2T_e^2 \tau_{Iee} T_h \tau_{IIhe} - 2T_e \tau_{Iee} T_h^2 \tau_{IIhe}} & 1 \leq E < 2 \\ \frac{T_e - e^{-3T_h + T_h E} T_e - T_h + e^{-3T_e + T_e E} T_h}{2T_e^2 \tau_{Iee} T_h \tau_{IIhe} - 2T_e \tau_{Iee} T_h^2 \tau_{IIhe}} & 2 \leq E < 3 \\ 0 & \text{else} \end{cases}$$

$$P_{14}(E | T_e = T_h) = \begin{cases} \frac{e^{-T \cdot E} (e^{T \cdot E} + e^T (-1 + T - T \cdot E))}{2T^2 \tau_{Iee} \tau_{IIhe}} & 1 \leq E < 2 \\ \frac{1 + e^{T(-3+E)} (-1 + T(-3+E))}{2T^2 \tau_{Iee} \tau_{IIhe}} & 2 \leq E < 3 \\ 0 & \text{else} \end{cases}$$

## Solution 15

**Description:** The electron creates a hole and the hole creates an electron.

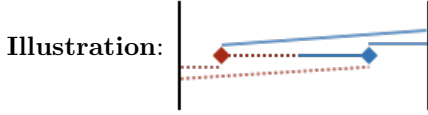

**Solutions:**

$$P_{15}(E | T_e \neq T_h) = \begin{cases} -\frac{e^{-((T_e + T_h)E)} (e^{2T_h + T_e E} - e^{2T_e + T_h E}) (-3 + E)}{\tau_{IIeh} (T_e - T_h) \tau_{IIhe}} & 2 \leq E < 3 \\ 0 & \text{else} \end{cases}$$

$$P_{15}(E | T_e = T_h) = \begin{cases} -\frac{e^{-T(-2+E)} (6 - 5E + E^2)}{\tau_{IIeh} \tau_{IIhe}} & 2 \leq E < 3 \\ 0 & \text{else} \end{cases}$$

## 5 Accessing the Solutions with Python

The single- $e^-h^+$ -pair solutions listed in Secs. 2–4 can be accessed through a Python file named “exponential\_CTH\_model\_1eh\_solutions.py” that is also provided as supplement material. The file contains a class called “single\_eh\_solutions” that initializes the CT and II parameters and provides the functions to return the single- $e^-h^+$ -pair solutions for the various event types. These functions are named “get\_surface\_events\_solutions”, “get\_bulk\_single\_charge\_event\_solutions”, and “get\_bulk\_eh\_pair\_event\_solutions”.

The return of these functions is a 2-d array containing the value of each unique solution evaluated at the energy grid points provided by the user. For surface events and bulk-single-charge events, the user must specify whether the initial charge is an electron or a hole. Furthermore for surface events and bulk- $e^-h^+$ -pair events, there is one solution that contains a Dirac delta function. In order to properly handle convolutions that may be performed using these solutions, the solution containing the Dirac delta function is kept as a separate object. Below shows an example of using this Python file to obtain the single- $e^-h^+$ -pair solutions.

```

import numpy as np
import exponential_CTII_model_1eh_solutions as ctii

# define an energy grid in the E_neh energy space:
Egrid = np.arange(0,4,0.01)

# define the fractional CT and II probabilities (the values shown here are arbitrary):
f_CTe=0.2 # probability for an electron to become trapped
f_CTh=0.1 # probability for a hole to become trapped
f_Ilee=0.01 # probability for an electron to create an unpaired electron
f_Ileh=0.02 # probability for an electron to create an unpaired hole
f_Ilhe=0.01 # probability for a hole to create an unpaired electron
f_Ilhh=0.05 # probability for a hole to create an unpaired hole

# initialize the single_eh_solutions object:
myctii=ctii.single_eh_solutions(f_CTe,f_CTh,f_Ilee,f_Ileh,f_Ilhe,f_Ilhh)

# obtain the solutions for surface events
# here, we need to specify if the initial charge is an electron or a hole
surface_delta_amp, surface_wo_delta = myctii.get_surface_event_solutions(Egrid,"e")

# calculate the total pdf for surface events:
surface_events_pdf_tot = np.sum(surface_wo_delta,axis=0)
surface_events_pdf_tot[np.where(Egrid==1)] += surface_delta_amp

# obtain the solutions for bulk-single-charge events
# here, we need to specify if the initial charge is an electron or a hole
bulkcharge_wo_delta = myctii.get_bulk_single_charge_event_solutions(Egrid,"e")

# calculate the total pdf for bulk-single-charge events:
bulkcharge_events_pdf_tot = np.sum(bulkcharge_wo_delta,axis=0)

# obtain the solutions for bulk-eh-pair events
bulkeh_delta_amp, bulkeh_wo_delta = myctii.get_bulk_eh_pair_event_solutions(Egrid)

# calculate the total pdf for bulk-eh-pair events:
bulkeh_events_pdf_tot = np.sum(bulkeh_wo_delta,axis=0)
bulkeh_events_pdf_tot[np.where(Egrid==1)] += bulkeh_delta_amp

```
